# Supplementary material for: On the Similarity between the Laplace and Neural Tangent Kernels
Source: arXiv:2007.01580 source file (2020-11-14)
Supplement: Supplementary file 1 [file citations_supp.tex]

@article{bordelon2020spectrum,
  title={Spectrum Dependent Learning Curves in Kernel Regression and Wide Neural Networks},
  author={Bordelon, Blake and Canatar, Abdulkadir and Pehlevan, Cengiz},
  journal={arXiv preprint arXiv:2002.02561},
  year={2020}
}
@article{sollich2002learning,
  title={Learning curves for Gaussian process regression: Approximations and bounds},
  author={Sollich, Peter and Halees, Anason},
  journal={Neural computation},
  volume={14},
  number={6},
  pages={1393--1428},
  year={2002},
  publisher={MIT Press}
}


@article{huang2020deep,
  title={Why Do Deep Residual Networks Generalize Better than Deep Feedforward Networks?--A Neural Tangent Kernel Perspective},
  author={Huang, Kaixuan and Wang, Yuqing and Tao, Molei and Zhao, Tuo},
  journal={arXiv preprint arXiv:2002.06262},
  year={2020}
}

@inproceedings{minh2006mercer,
  title={Mercer’s theorem, feature maps, and smoothing},
  author={Minh, Ha Quang and Niyogi, Partha and Yao, Yuan},
  booktitle={International Conference on Computational Learning Theory},
  pages={154--168},
  year={2006},
  organization={Springer}
}
@article{novak2018bayesian,
  title={Bayesian deep convolutional networks with many channels are gaussian processes},
  author={Novak, Roman and Xiao, Lechao and Lee, Jaehoon and Bahri, Yasaman and Yang, Greg and Hron, Jiri and Abolafia, Daniel A and Pennington, Jeffrey and Sohl-Dickstein, Jascha},
  journal={arXiv preprint arXiv:1810.05148},
  year={2018}
}
@article{li2019enhanced,
  title={Enhanced Convolutional Neural Tangent Kernels},
  author={Li, Zhiyuan and Wang, Ruosong and Yu, Dingli and Du, Simon S and Hu, Wei and Salakhutdinov, Ruslan and Arora, Sanjeev},
  journal={arXiv preprint arXiv:1911.00809},
  year={2019}
}
@article{narcowich2007approximation,
  title={Approximation power of RBFs and their associated SBFs: a connection},
  author={Narcowich, Francis J and Sun, Xinping and Ward, Joseph D},
  journal={Advances in Computational Mathematics},
  volume={27},
  number={1},
  pages={107--124},
  year={2007},
  publisher={Springer}
}
@book{stein2016introduction,
  title={Introduction to Fourier analysis on Euclidean spaces (PMS-32)},
  author={Stein, Elias M and Weiss, Guido},
  volume={32},
  year={2016},
  publisher={Princeton university press}
}
@article{bach2017breaking,
  title={Breaking the curse of dimensionality with convex neural networks},
  author={Bach, Francis},
  journal={The Journal of Machine Learning Research},
  volume={18},
  number={1},
  pages={629--681},
  year={2017},
  publisher={JMLR. org}
}
@inproceedings{bietti2019inductive,
  title={On the inductive bias of neural tangent kernels},
  author={Bietti, Alberto and Mairal, Julien},
  booktitle={Advances in Neural Information Processing Systems},
  pages={12873--12884},
  year={2019}
}

@article{narcowich2002scattered,
  title={Scattered data interpolation on spheres: error estimates and locally supported basis functions},
  author={Narcowich, Francis J and Ward, Joseph D},
  journal={SIAM Journal on Mathematical Analysis},
  volume={33},
  number={6},
  pages={1393--1410},
  year={2002},
  publisher={SIAM}
}

@inproceedings{jacot2018neural,
  title={Neural tangent kernel: Convergence and generalization in neural networks},
  author={Jacot, Arthur and Gabriel, Franck and Hongler, Cl{\'e}ment},
  booktitle={Advances in neural information processing systems},
  pages={8571--8580},
  year={2018}
}

@inproceedings{arora2019exact,
  title={On exact computation with an infinitely wide neural net},
  author={Arora, Sanjeev and Du, Simon S and Hu, Wei and Li, Zhiyuan and Salakhutdinov, Russ R and Wang, Ruosong},
  booktitle={Advances in Neural Information Processing Systems},
  pages={8139--8148},
  year={2019}
}

@inproceedings{daniely2016toward,
  title={Toward deeper understanding of neural networks: The power of initialization and a dual view on expressivity},
  author={Daniely, Amit and Frostig, Roy and Singer, Yoram},
  booktitle={Advances In Neural Information Processing Systems},
  pages={2253--2261},
  year={2016}
}
@inproceedings{ronen2019convergence,
  title={The convergence rate of neural networks for learned functions of different frequencies},
  author={Basri, Ronen and Jacobs, David and Kasten, Yoni and Kritchman, Shira},
  booktitle={Advances in Neural Information Processing Systems},
  pages={4763--4772},
  year={2019}
}

@inproceedings{cho2009kernel,
  title={Kernel methods for deep learning},
  author={Cho, Youngmin and Saul, Lawrence K},
  booktitle={Advances in neural information processing systems},
  pages={342--350},
  year={2009}
}

@book{watson1995treatise,
  title={A treatise on the theory of Bessel functions},
  author={Watson, George Neville},
  year={1966},
  publisher={Cambridge university press}
}
@book{saitoh2016theory,
  title={Theory of reproducing kernels and applications},
  author={Saitoh, Saburou and Sawano, Yoshihiro},
  year={2016},
  publisher={Springer}
}

@book{paulsen_raghupathi_2016, place={Cambridge}, series={Cambridge Studies in Advanced Mathematics}, title={An Introduction to the Theory of Reproducing Kernel Hilbert Spaces}, DOI={10.1017/CBO9781316219232}, publisher={Cambridge University Press}, author={Paulsen, Vern I. and Raghupathi, Mrinal}, year={2016}, collection={Cambridge Studies in Advanced Mathematics}}

@misc{basriNonuniform,
    title={Frequency Bias in Neural Networks for Input of Non-Uniform Density},
    author={Ronen Basri and Meirav Galun and Amnon Geifman and David Jacobs and Yoni Kasten and Shira Kritchman},
    year={2020},
    eprint={2003.04560},
    archivePrefix={arXiv},
    primaryClass={cs.LG}
}

@article{yang2019scaling,
  title={Scaling limits of wide neural networks with weight sharing: Gaussian process behavior, gradient independence, and neural tangent kernel derivation},
  author={Yang, Greg},
  journal={arXiv preprint arXiv:1902.04760},
  year={2019}
}

@article{ghorbani2019linearized,
  title={Linearized two-layers neural networks in high dimension},
  author={Ghorbani, Behrooz and Mei, Song and Misiakiewicz, Theodor and Montanari, Andrea},
  journal={arXiv preprint arXiv:1904.12191},
  year={2019}
}

@article{belkin2018understand,
  title={To understand deep learning we need to understand kernel learning},
  author={Belkin, Mikhail and Ma, Siyuan and Mandal, Soumik},
  journal={arXiv preprint arXiv:1802.01396},
  year={2018}
}

@article{liang2018just,
  title={Just interpolate: Kernel" ridgeless" regression can generalize},
  author={Liang, Tengyuan and Rakhlin, Alexander},
  journal={arXiv preprint arXiv:1808.00387},
  year={2018}
}

@inproceedings{belkin2018overfitting,
  title={Overfitting or perfect fitting? risk bounds for classification and regression rules that interpolate},
  author={Belkin, Mikhail and Hsu, Daniel J and Mitra, Partha},
  booktitle={Advances in neural information processing systems},
  pages={2300--2311},
  year={2018}
}

@article{aronszajn1950theory,
  title={Theory of reproducing kernels},
  author={Aronszajn, Nachman},
  journal={Transactions of the American mathematical society},
  volume={68},
  number={3},
  pages={337--404},
  year={1950},
  publisher={JSTOR}
}

@article{baldi2014searching,
  title={Searching for exotic particles in high-energy physics with deep learning},
  author={Pierre Baldi, Peter Sadowski, and Daniel Whiteson},
  journal={Nature communications},
  Volume={5},
  year={2014}
}
@book{neal2012bayesian,
  title={Bayesian learning for neural networks},
  author={Neal, Radford M},
  volume={118},
  year={2012},
  publisher={Springer Science \& Business Media}
}
@inproceedings{williams1997computing,
  title={Computing with infinite networks},
  author={Williams, Christopher KI},
  booktitle={Advances in neural information processing systems},
  pages={295--301},
  year={1997}
}

@article{jetter1999error,
  title={Error estimates for scattered data interpolation on spheres},
  author={Jetter, Kurt and St{\~A}{\c{k}}ckler, Joachim and Ward, Joseph},
  journal={Mathematics of Computation},
  volume={68},
  number={226},
  pages={733--747},
  year={1999}
}


@book{GammaExponential,
  title={Gaussian Processes for Machine Learning},
  author={Carl Edward Rasmussen and Christopher K. I. Williams},
  pages={86-87},
  year={2006},
  publisher={MIT Press}
}

@incollection{Rahimi2007,
title = {Random Features for Large-Scale Kernel Machines},
author = {Ali Rahimi and Recht, Benjamin},
booktitle = {Advances in Neural Information Processing Systems 20},
editor = {J. C. Platt and D. Koller and Y. Singer and S. T. Roweis},
pages = {1177--1184},
year = {2007}
}

@article{Genton2001,
author = {Genton, Marc G.},
journal = {Journal of Machine Learning Research},
pages = {299-312},
title = {Classes of Kernels for Machine Learning: A Statistics Perspective.},
  volume = {2},
  year = {2001}
}


@InProceedings{allen-zhu2019,
  title = {A Convergence Theory for Deep Learning via Over-Parameterization},
  author = 	 {Allen-Zhu, Zeyuan and Li, Yuanzhi and Song, Zhao},
  booktitle = {Proceedings of the 36th International Conference on Machine Learning},
  pages = 	 {242--252},
  year = 	 {2019},
  editor = 	 {Chaudhuri, Kamalika and Salakhutdinov, Ruslan},
  volume = 	 {97}
}

@inproceedings{
Arora2020Harnessing,
title={Harnessing the Power of Infinitely Wide Deep Nets on Small-data Tasks},
author={Sanjeev Arora and Simon S. Du and Zhiyuan Li and Ruslan Salakhutdinov and Ruosong Wang and Dingli Yu},
booktitle={International Conference on Learning Representations},
year={2020}
}

@article{arora2019fine,
  title={Fine-grained analysis of optimization and generalization for overparameterized two-layer neural networks},
  author={Arora, Sanjeev and Du, Simon S and Hu, Wei and Li, Zhiyuan and Wang, Ruosong},
  journal={arXiv preprint arXiv:1901.08584},
  year={2019}
}

@techreport{micchelli1979design,
  title={Design Problems for Optimal Surface Interpolation.},
  author={Micchelli, Charles A and Wahba, Grace},
  year={1979},
  institution={WISCONSIN UNIV-MADISON DEPT OF STATISTICS}
}

@article{cao2019towards,
  title={Towards Understanding the Spectral Bias of Deep Learning},
  author={Cao, Yuan and Fang, Zhiying and Wu, Yue and Zhou, Ding-Xuan and Gu, Quanquan},
  journal={arXiv preprint arXiv:1912.01198},
  year={2019}
}

@article{yang2019fine,
  title={A fine-grained spectral perspective on neural networks},
  author={Yang, Greg and Salman, Hadi},
  journal={arXiv preprint arXiv:1907.10599},
  year={2019}
}

@article{kimeldorf1970correspondence,
  title={A correspondence between Bayesian estimation on stochastic processes and smoothing by splines},
  author={Kimeldorf, George S and Wahba, Grace},
  journal={The Annals of Mathematical Statistics},
  volume={41},
  number={2},
  pages={495--502},
  year={1970},
  publisher={JSTOR}
}

@incollection{Bo2010nips,
title = {Kernel Descriptors for Visual Recognition},
author = {Liefeng Bo and Xiaofeng Ren and Dieter Fox},
booktitle = {Advances in Neural Information Processing Systems 23},
editor = {J. D. Lafferty and C. K. I. Williams and J. Shawe-Taylor and R. S. Zemel and A. Culotta},
pages = {244--252},
year = {2010}
}

@incollection{Mairal2014conv,
title = {Convolutional Kernel Networks},
author = {Mairal, Julien and Koniusz, Piotr and Harchaoui, Zaid and Schmid, Cordelia},
booktitle = {Advances in Neural Information Processing Systems 27},
editor = {Z. Ghahramani and M. Welling and C. Cortes and N. D. Lawrence and K. Q. Weinberger},
pages = {2627--2635},
year = {2014}
}

@article{fernandez2014we,
  title={Do we need hundreds of classifiers to solve real world classification problems?},
  author={Fern{\'a}ndez-Delgado, Manuel and Cernadas, Eva and Barro, Sen{\'e}n and Amorim, Dinani},
  journal={The journal of machine learning research},
  volume={15},
  number={1},
  pages={3133--3181},
  year={2014},
  publisher={JMLR. org}
}



@inproceedings{rudi2017falkon,
  title={Falkon: An optimal large scale kernel method},
  author={Rudi, Alessandro and Carratino, Luigi and Rosasco, Lorenzo},
  booktitle={Advances in Neural Information Processing Systems},
  pages={3888--3898},
  year={2017}
}

@article{demvsar2006statistical,
  title={Statistical comparisons of classifiers over multiple data sets},
  author={Dem{\v{s}}ar, Janez},
  journal={Journal of Machine learning research},
  volume={7},
  number={Jan},
  pages={1--30},
  year={2006}
}


@article{fan2020spectra,
  title={Spectra of the Conjugate Kernel and Neural Tangent Kernel for linear-width neural networks},
  author={Fan, Zhou and Wang, Zhichao},
  journal={arXiv preprint arXiv:2005.11879},
  year={2020}
}
@article{chapelle2007training,
  title={Training a support vector machine in the primal},
  author={Chapelle, Olivier},
  journal={Neural computation},
  volume={19},
  number={5},
  pages={1155--1178},
  year={2007},
  publisher={MIT Press}
}

@article{bertin2011million,
  title={The million song dataset},
  author={Bertin-Mahieux, Thierry and Ellis, Daniel PW and Whitman, Brian and Lamere, Paul},
  year={2011}
}

@article{cho2011analysis,
  title={Analysis and extension of arc-cosine kernels for large margin classification},
  author={Cho, Youngmin and Saul, Lawrence K},
  journal={arXiv preprint arXiv:1112.3712},
  year={2011}
}

@inproceedings{dai2014scalable,
  title={Scalable kernel methods via doubly stochastic gradients},
  author={Dai, Bo and Xie, Bo and He, Niao and Liang, Yingyu and Raj, Anant and Balcan, Maria-Florina F and Song, Le},
  booktitle={Advances in Neural Information Processing Systems},
  pages={3041--3049},
  year={2014}
}

@book{scholkopf2001learning,
  title={Learning with kernels: support vector machines, regularization, optimization, and beyond},
  author={Scholkopf, Bernhard and Smola, Alexander J},
  year={2001},
  publisher={MIT press}
}

@article{Difan2020,
  title={Gradient descent optimizes over-parameterized deep ReLU networks},
  author={Difan Zou and Yuan Cao and Dongruo Zhou and Quanquan Gu},
  journal={Machine Learning},
  volume={109},
  year={2020},
  pages={467--492}
  }
  
@article{matthews2018gaussian,
  title={Gaussian process behaviour in wide deep neural networks},
  author={Matthews, Alexander G de G and Rowland, Mark and Hron, Jiri and Turner, Richard E and Ghahramani, Zoubin},
  journal={arXiv preprint arXiv:1804.11271},
  year={2018}
}  
@article{lee2017deep,
  title={Deep neural networks as gaussian processes},
  author={Lee, Jaehoon and Bahri, Yasaman and Novak, Roman and Schoenholz, Samuel S and Pennington, Jeffrey and Sohl-Dickstein, Jascha},
  journal={arXiv preprint arXiv:1711.00165},
  year={2017}
}

@article{gallier2009notes,
  title={Notes on spherical harmonics and linear representations of Lie groups},
  author={Gallier, Jean},
  journal={preprint},
  year={2009}
}

@article{kanagawa2018gaussian,
  title={Gaussian processes and kernel methods: A review on connections and equivalences},
  author={Kanagawa, Motonobu and Hennig, Philipp and Sejdinovic, Dino and Sriperumbudur, Bharath K},
  journal={arXiv preprint arXiv:1807.02582},
  year={2018}
}

@misc{chen2020deep,
      title={Deep Neural Tangent Kernel and Laplace Kernel Have the Same RKHS}, 
      author={Lin Chen and Sheng Xu},
      year={2020},
      eprint={2009.10683},
      archivePrefix={arXiv},
      primaryClass={cs.LG}
}
